# Supplementary material for: Multi-Modality Driven LoRA for Adverse Condition Depth Estimation
Source: arXiv:2412.20162 source file (2024-12-28)
Supplement: Supplementary file 1 [file X_suppl.tex]

\clearpage
\setcounter{page}{1}
\maketitlesupplementary

\textbf{Evaluation metrics.}
These error metrics are defined as: 

\begin{itemize}
\item Abs relative error(absREL):$\frac{1}{N} \sum_{i=1}^{N} \frac{|y_{i}-\hat{y}_{i}|}{y_i}$;

\item Root mean squared error(RMSE): $\sqrt{\frac{1}{N} \sum_{i=1}^{N} (\hat{y}_i - y_i)^2}$;

\item Squared Relative Difference (sqRel): $\frac{1}{N} \sum_{i=1}^{N} \left( \frac{\hat{y}_i - y_i}{y_i} \right)^2$;

\item Accuracy with threshold t: percentage(\%) of $\hat{y}_i$, subject to max ($\frac{\hat{y}_i}{y_i}$, $\frac{y_i}{\hat{y_i}}$) = d $<$ $1.25^k$ for k=1,2,3;
\end{itemize}
where the $\hat{y}_i$ and ${y}_i$ are the ground-truth depth and the estimated depth at pixel $i$ respectively. N is the total number of pixels of the test images.

\begin{table*}[t]
\scriptsize
\centering

\caption{Ablation study results of Prompt Driven Domain Alignment (PDDA) and Consistent Visual-Text Contrastive Learning (VTCCL) on the RobotCar test set. The performance of the proposed MMD-LoRA method with or without PDDA and VTCCL are reported.
}
\vspace{-0.3cm}
\setlength{\tabcolsep}{3.5mm}{
\begin{tabular}{c c c c c c c c c c}
\toprule
\multirow{2}{*}{PDDA} &\multirow{2}{*}{VTCCL} &\multicolumn{4}{c}{day-RobotCar} & \multicolumn{4}{c}{night-RobotCar} \\ 
\cmidrule(r){3-6} \cmidrule(r){7-10}
& & absREL($\downarrow$)& sqREL($\downarrow$) & RMSE($\downarrow$) & $d_1$($\uparrow$) & absREL($\downarrow$)& sqREL($\downarrow$) & RMSE($\downarrow$) & $d_1$($\uparrow$) \\ 
\midrule
\texttimes & \texttimes &0.0794	&0.322	&\textbf{2.188}	&92.53	&0.0935	&0.417	&2.774	&88.50 \\ 
\texttimes & \checkmark &\textbf{0.0777}	&\textbf{0.311}	&2.193	&92.53&	0.0887	&0.391	&2.695	&89.02\\ 
\checkmark & \checkmark &0.0796	&0.324&	2.191	&\textbf{92.56}	&\textbf{0.0881}	&\textbf{0.385}&\textbf{2.643}	&\textbf{89.33}\\ 
\bottomrule
\end{tabular}
}
\vspace{-0.3cm}
\label{ablation_tab_robotcar}
\end{table*}

\begin{table*}[t]
\scriptsize
\centering

\caption{The depth estimation performance in different threshold value ratios($\lambda$) of Visual-Text Consistent Contrastive Learning (VTCCL) for each weather. 
Adapting $\lambda_0$:$\lambda_1$:$\lambda_2$=1:0.1:1 and $\lambda_0$:$\lambda_1$=1:0.05 give the best performance overall on the nuScenes validation set and RobotCar test set.}
\vspace{-0.3cm}
\setlength{\tabcolsep}{3.5mm}{
\begin{tabular}{c c c c c c c c c c c c}
\toprule
\multirow{2}{*}{$\lambda_{0}$} & \multirow{2}{*}{$\lambda_{1}$} & \multirow{2}{*}{$\lambda_{2}$} & \multicolumn{3}{c}{day-clear} & \multicolumn{3}{c}{night} & \multicolumn{3}{c}{day-rain} \\ 
\cmidrule(r){4-6}  \cmidrule(r){7-9} \cmidrule(r){10-12}
&  &  & absREL($\downarrow$) & RMSE($\downarrow$) & d1($\uparrow$) & absREL($\downarrow$) & RMSE($\downarrow$) & d1($\uparrow$) & absREL($\downarrow$) & RMSE($\downarrow$) & d1($\uparrow$) \\ 
\midrule
1 & 1 & 1 & 0.0711  & 3.243  &  96.56	& 0.1772   & 8.071     & 74.39	& 0.0731  &  3.457 &   95.38\\ 
\textbf{1} & \textbf{0.1} & \textbf{1} &\textbf{0.0690}  &\textbf{3.192}  & \textbf{96.46}	&\textbf{0.1545}  & \textbf{7.127}   &\textbf{79.96}	&\textbf{0.0740}  & \textbf{3.417}   &\textbf{95.37} \\ 
1 & 1 & 0.1  &0.0710 & 3.275  & 96.05&	0.1669   &7.756    & 76.92  &	0.0792  & 3.589  & 94.25\\ 
1 & 1 & ---  &0.0781    &  2.182 &    92.60	&0.0861     &2.707    & 89.24  &---  & ---  & ---\\ 
1 & 0.1 & ---  &0.0781   &  2.191    & 92.55&	0.0886   &2.689    & 89.04  &	---  & ---  & ---\\ 
\textbf{1} & \textbf{0.05} & --- &\textbf{0.0796}  &\textbf{2.191}  & \textbf{92.56}	&\textbf{0.0881}  &\textbf{2.643}   &\textbf{89.33}  &	---  & ---  & ---\\ 
\bottomrule
\end{tabular}
}
\label{lambda-comparsion1}
\vspace{-0.3cm}
\end{table*}

\begin{figure*}[!t]
\centering
\includegraphics[width=1.0\textwidth]{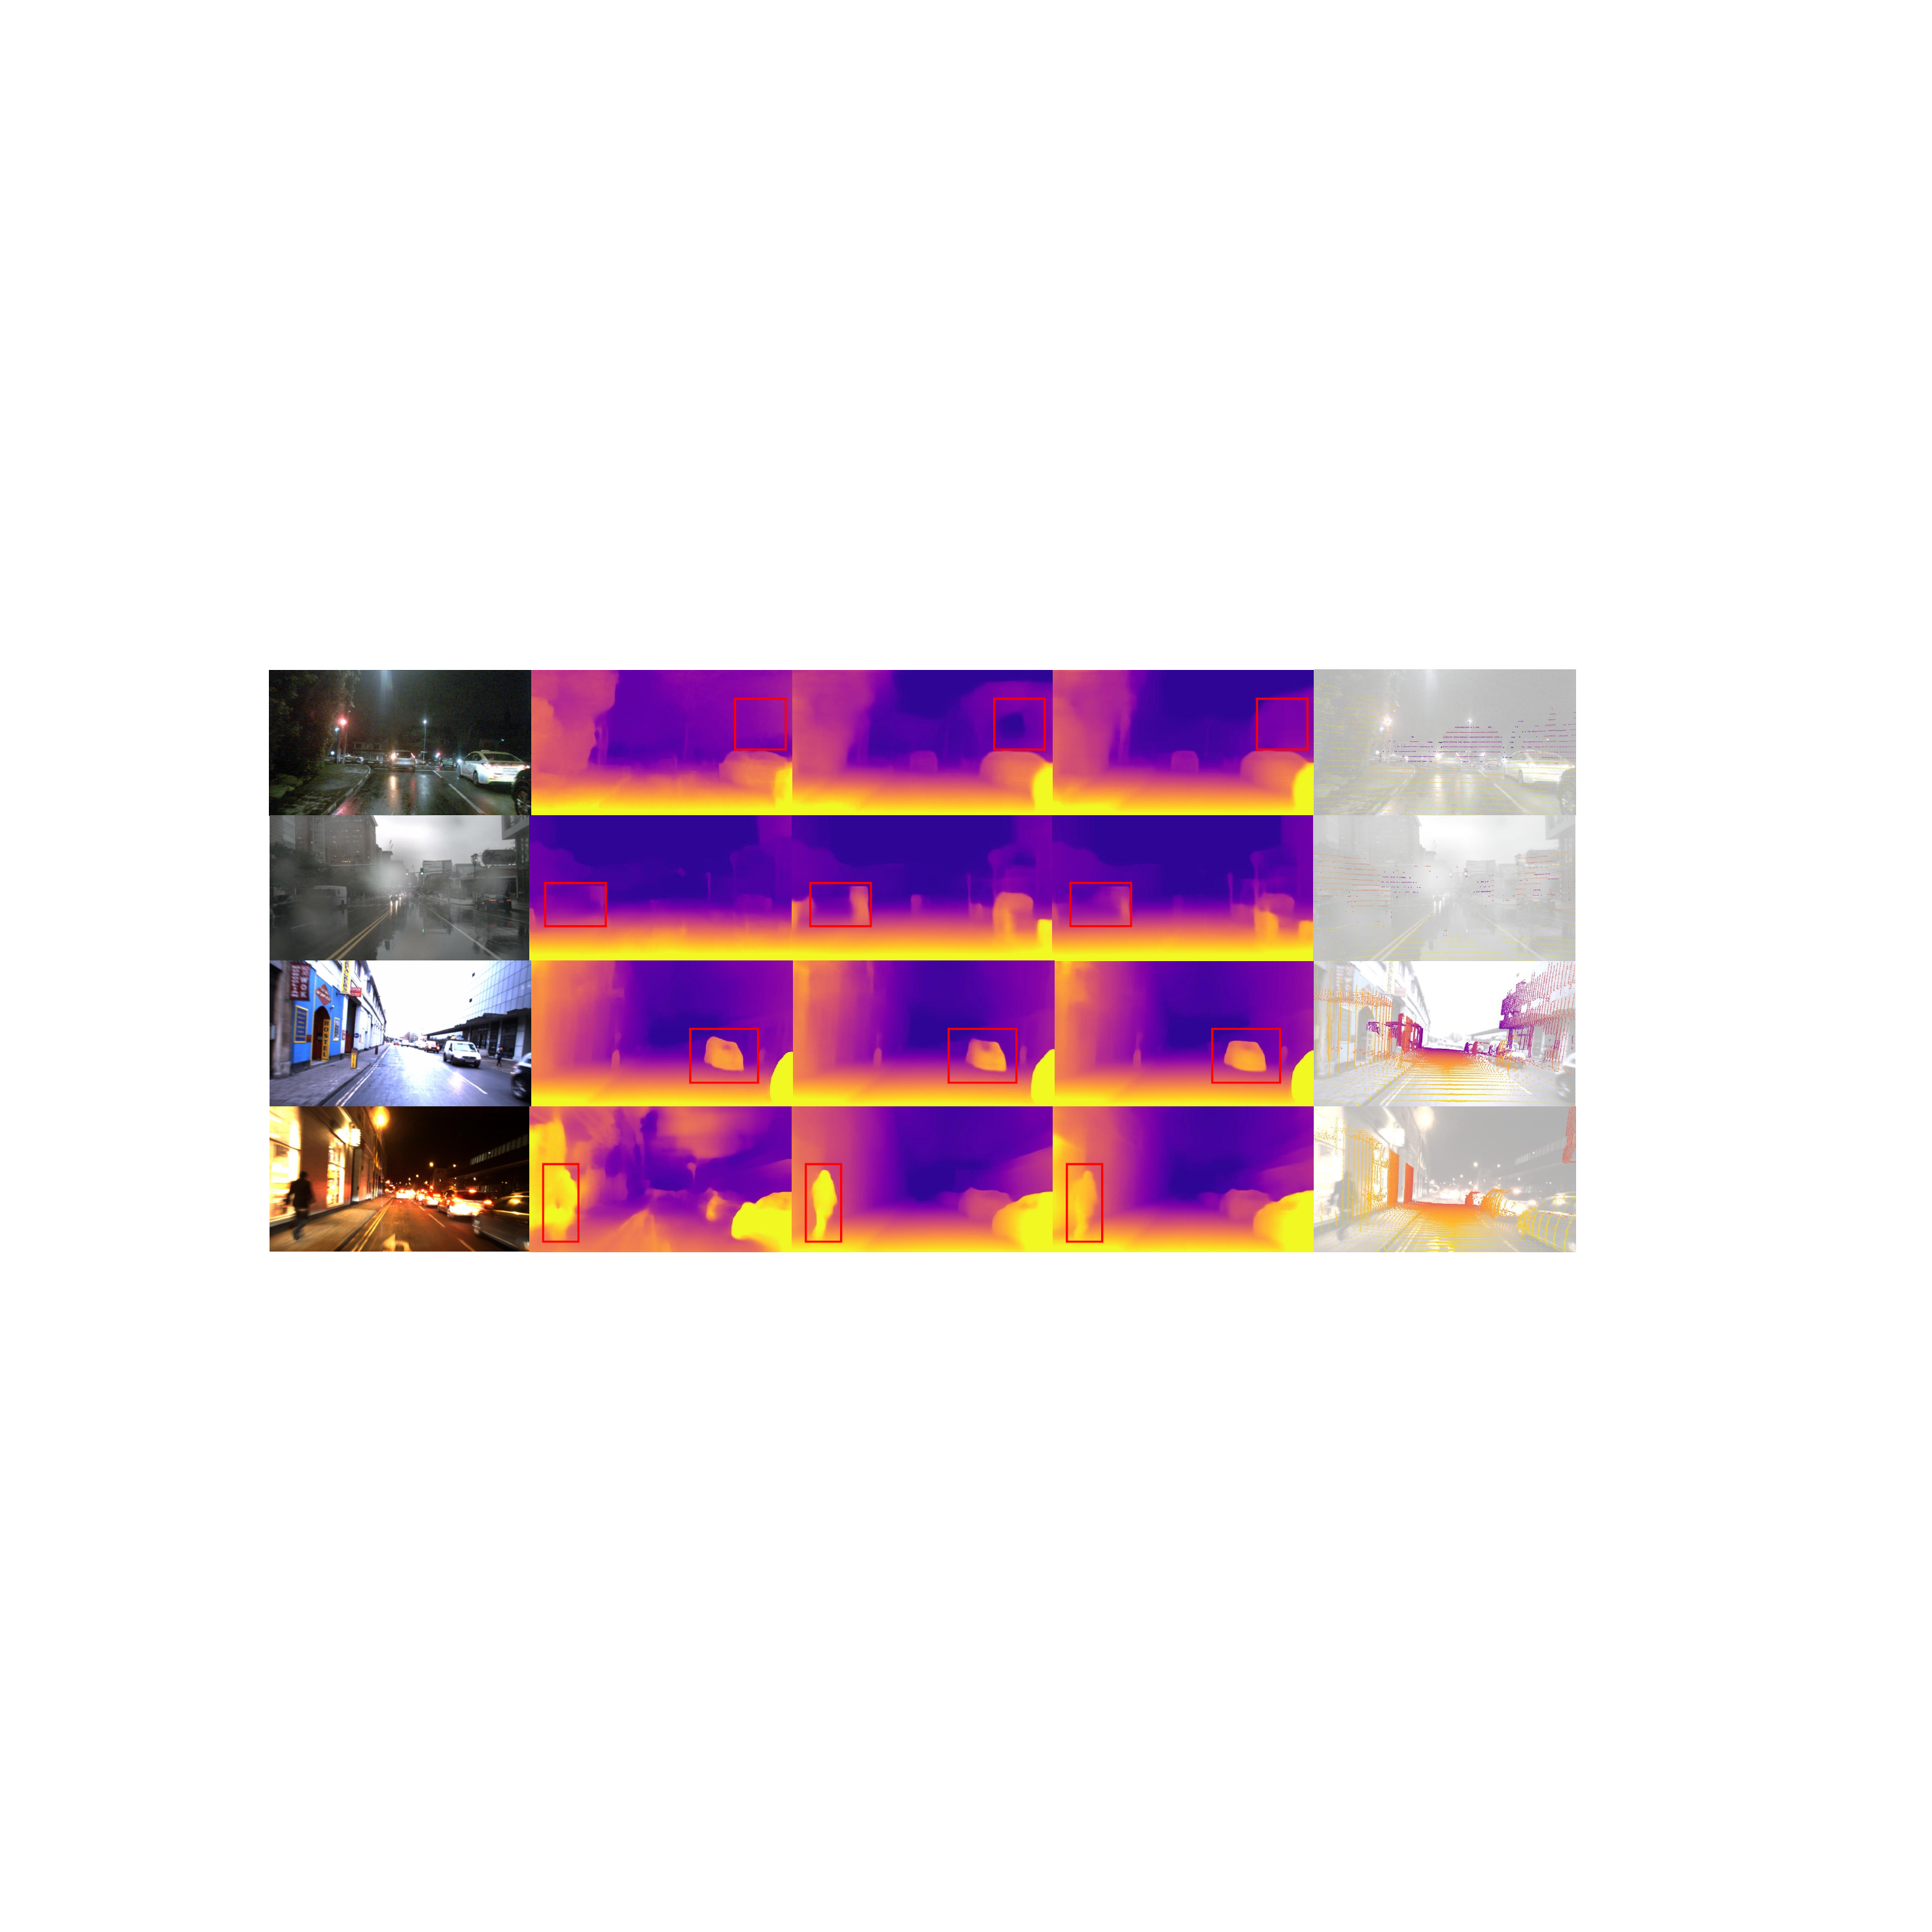}
\caption{Qualitative results of our proposed MMD-LoRA and the previous SOTA depth estimation method on the nuScenes validation sets and Robotcar test set. 
The first column denotes the original image. The second column, third column and fourth column denote the depth estimation results of Monodepth2, md4allDD and ours MMD-LoRA respectively. 
The final column indicates the ground-truth depth maps.
}
\label{vis-all-supp}
\end{figure*}

\begin{figure*}[!t]
\centering
\includegraphics[width=1.0\textwidth]{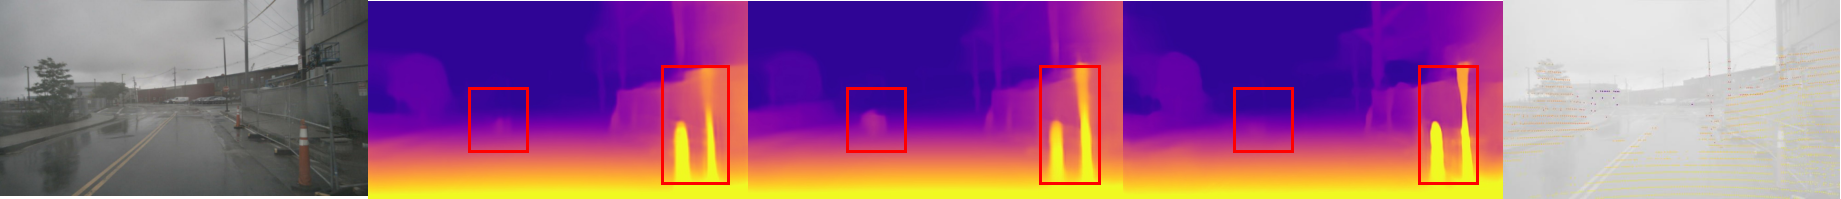}
\caption{Ablation visualization of our proposed MMD-LoRA with PDDA and VTCCL.
The first column denotes the original image. The second, third and fourth column denote baseline(\ie EVP~\cite{EVP}), MMD-LoRA with PDDA, MMD-LoRA with PDDA and VTCCL. 
The final column indicates the ground-truth depth maps.
}
\label{vis-xiaorong-supp}
\end{figure*}

\textbf{Training step loss.} 
During the training phase, we inject the trained MMD-LoRA into the 'q', 'k', 'v', and 'proj' layers of the self-attention in the image encoder.
When encountering rare weather conditions, we introduce the corresponding target-domain text descriptions to further pre-train MMD-LoRA.
Throughout training, the baseline depth estimator leverages the image captions to capture semantic information about complex road scenarios in the real world. 
The trained MMD-LoRA, integrated with the image encoder, estimates the unseen target-domain visual representations while extracting source-domain visual representations. 
The diverse visual representations and text embeddings from the image captions are utilized through cross-attention maps to provide explicit guidance for depth estimation tasks.
The decoder features of the denoising U-Net then feed into the Inverse Multi-Attentive Feature Refinement (IMFAR), which captures enhanced visual representations. Finally, the depth estimation decoder generates the predicted depth map.
% In the training step, we inject the trained MMD-LoRA into ’q’,’k’,’v’, ’proj’ layers of self-attention in the image encoder and further optimize baseline depth estimator(\eg EVP~\cite{EVP}).
% Once encountering rare weather conditions, we only introduce the target-domain text description to further pre-train MMD-LoRA.
% During the training step, the baseline depth estimator utilizes the image caption to capture the semantic information of complex road scenario in the real world, and trained MMD-LoRA with image encoder estimates the unseen target-domain visual representations and extracts source-domain visual representation.
% The various visual representations and text embeddings of image captions utilize cross-attention maps to provide explicit guidance for depth estimation tasks. 
% Then, the denoising U-Net’s decoder features feed on the Inverse Multi-Attentive Feature Refinement (IMFAR) to capture enhanced visual representation and the depth estimation decoder outputs the predicted depth map.
The depth estimator is then trained with the pixel-wise depth loss during the training step:
\begin{equation}
\label{gongshi7}
\begin{aligned}
\displaystyle 
L_{train} = \sqrt{\frac{1}{T} \sum_i g_i^2 -\frac{\mu}{T^2} (\sum_i g_i)^2}
\end{aligned}
\end{equation}
where $g_i$=$log~\hat{d_i} - log~d_i$, $\hat{d_i}$ denotes the predicted depth and $d_i$ denotes the ground-truth depth at pixel $i$ respectively. T denotes the number of pixels having valid ground-truth values.

\textbf{Ablation study on the RobotCar.}
To further validate the effectiveness and robustness of our proposed PDDA and VTCCL, we evaluate the performance of MMD-LoRA's components. 
As shown in Tab.~\ref{ablation_tab_robotcar}, the results demonstrate that MMD-LoRA with only PDDA achieves a $d_1$ score of 89.02\% for nighttime conditions, significantly outperforming the baseline depth estimator.
By incorporating VTCCL, the performance of MMD-LoRA further increases from 89.02\% to 89.33\%, highlighting the added benefits of VTCCL in enhancing the robustness of our approach. 
Across all tested conditions, the proposed MMD-LoRA consistently outperforms the baseline depth estimator, achieving these improvements without relying on target-domain images, thus validating its efficacy and generalization capability.

% To validate the effectiveness and robustness of our proposed PDDA and VTCCL further, we explore the MMD-LoRA performance using PDDA and VTCCL. 
% As shown in Tab.~\ref{ablation_tab_robotcar}, we can observe that the MMD-LoRA using only PDDA achieves 89.02\% in $d_1$ for night compared with the baseline depth estimator.
% By further introducing the VTCCL, the MMD-LoRA performance increases from 89.02\% to 89.33\%, which further validates the effectiveness and robustness of our proposed MMD-LoRA.
% Across all tested conditions, the proposed MMD-LoRA method significantly improves over the baseline depth estimator on which we applied it, without the need for target-domain images. 

% We conduct the ablation study on the RobotCar dataset as shown in Table~\ref{ablation_tab_robotcar}. Our MMD-LoRA with the PDDA and VTCCL deliver improvements for the EVP baseline(\eg $d_1$ from 92.53\% to 92.56\% in the day, $d_1$ from 88.50\% to 89.33\% in the night). 
% Across all tested conditions, the proposed MMD-LoRA method significantly improves over EVP on which we applied it, without the need for specialized translated image generation. 

% \textbf{Analysis of contrastive learning weight coefficients $\lambda$ for each weather condition in VTCCL}. 
\textbf{Analysis of contrastive learning weight coefficients in VTCCL}. 
To determine the optimal weight coefficients for contrastive learning, we evaluate the performance of MMD-LoRA on the nuScenes validation set and the RobotCar test set under various settings. As shown in Table~\ref{lambda-comparsion1}, the best scaling factors are observed to be
$\lambda_0$: $\lambda_1$:$\lambda_2$=1:0.1:1 on the nuScenes validation set while $\lambda_0$: $\lambda_1$=1:0.05 on the RobotCar test set.
The results indicate that setting $\lambda=1$ is most effective for daytime conditions (e.g., day-clear, day-rain on the nuScenes dataset, and day-clear on the RobotCar dataset), while lower values of $\lambda$are better suited for nighttime scenarios (e.g., 
$\lambda=0.05$for night-RobotCar and 
$\lambda=0.1$ for night-nuScenes). 
These findings highlight the importance of adaptive weight coefficients for optimizing MMD-LoRA under varying environmental conditions.

% In VTCCL, to make clear how to tune the contrastive learning weight coefficients $\lambda$, we compare the performance of MMD-LoRA on the nuScenes validation set and the RobotCar test set under the setting of various $\lambda$.
% As shown in Table~\ref{lambda-comparsion1}, we observe that the best scale factor $\lambda_0$: $\lambda_1$:$\lambda_2$=1:0.1:1 on the nuScenes validation set and $\lambda_0$ :$\lambda_1$=1:0.05 on the RobotCar test set when using various $\lambda$(\ie 1:1:1, 1:0.1:1, 1:1:0.1 on the nuScenes validation set and 1:1, 1:0.1, 1:0.05 on the RobotCar test set). 
% Based on the above experimental results, we can conclude that the coefficient is set to 1 for adapting the daytime(\eg day-clear, day-rain on the nuScenes dataset and day-clear on the RobotCar dataset) and the coefficient is set to less than 1 for the nighttime(\eg 0.05 on the night-RobotCar and 0.1 on the night-nuScenes).

\textbf{Qualitative results and ablation visualization.}
As shown in Fig~\ref{vis-all-supp}, we compare our MMD-LoRA with Monodepth and md4all on the sunny condition and particularly challenging night/rain samples due to the extreme darkness levels, the high amount of floored reflections. 
Our MMD-LoRA delivered overall sharper and more accurate estimates, as can be seen for the thin structures(e.g. person, and car), as well as the complete vehicles. For example, our MMD-LoRA correctly recovers the 'holes' in the sky, which is particularly hard to see.

Meanwhile, we further expand the visualization results of ablation experiments on the nuScenes validation set in Eq.~\ref{ablation_tab_nusence}.
As shown in Fig.~\ref{vis-xiaorong-supp}, EVP struggles to the standing pillar outline. Compared with the EVP, PDDA delivered a sharp estimation for the standing pillar. However, we observed that EVP and MMD-LoRA regard the floored reflection as an object and estimate the depth value of 'object' as shown in the red box of Fig.~\ref{vis-xiaorong-supp}. The above phenomenon seriously affects the safety of autonomous driving in adverse condition.
The MMD-LoRA with VTCCL not only enriched the object boundary, but also eliminated the impact of this reflection.

% 消融20241120
% sunny  0.0692   3.1967   96.65   0.2290  9.7442  63.3    0.0762   3.4931  95.39
% sunny and night  0.0818  4.1347  93.61
% 0.1625  7.1668   79.98
% 0.0843  3.6674  93.37

% sunny and rain   0.0627  2.9836   96.76  0.2264  9.4543   64.00       0.07   3.2266   95.73  

% all 0.0690  3.192  96.46  0.1545  7.127  
%79.96  0.0740  3.417  95.37  

\begin{table*}[t]
\scriptsize
\centering
\caption{Evaluation on the nuScenes validation set. 
The bold entries denote that our MMD-LoRA surpasses previous SOTA results.}
\vspace{-0.2cm}

\begin{tabular}{c c c c c c c c c c c c}
\toprule
\multicolumn{3}{c}{VTCCL in Eq.~\ref{gongshi5}} &\multicolumn{3}{c}{day-clear-nuScenes} &\multicolumn{3}{c}{night-nuScenes} &\multicolumn{3}{c}{day-rain-nuScenes} \\ 
\cmidrule(r){1-3}  \cmidrule(r){4-6} \cmidrule(r){7-9} \cmidrule(r){10-12}
day-clear &night &day-rain & absREL($\downarrow$) & RMSE($\downarrow$) & $d_1$($\uparrow$) & absREL($\downarrow$) & RMSE($\downarrow$) & $d_1$($\uparrow$) & absREL($\downarrow$) & RMSE($\downarrow$) & $d_1$($\uparrow$) \\ 
\midrule
\texttimes & \texttimes & \texttimes  &0.0689	&3.118	&96.09	&0.1426 &7.742	&80.46	&0.084	&3.565	&94.09 \\
\checkmark & \texttimes & \texttimes	&0.0692   &3.197   &96.65  & 0.2290  &9.744  &63.30    &0.076   &3.493  &95.39\\
\checkmark & \checkmark & \texttimes	&0.0818  &4.135 & 93.61 &0.1625  &7.167   &79.98 &0.084  &3.667  &93.37  \\
\checkmark & \texttimes & \checkmark	&0.0627  &2.984   &96.76  &0.2264  &9.454   &64.00       &0.070   &3.227   &95.73  \\
\checkmark & \checkmark & \checkmark	&0.0690  &3.192  &96.46 & 0.1545  &7.127  
&79.96  &0.074  &3.417  &95.37\\
\bottomrule
\end{tabular}
\label{tianqi_xiaorong}
\end{table*}

\textbf{Influence of combining various weather in VTCCL.}
As shown in Table~\ref{tianqi_xiaorong}, we analyze the impact of incorporating various weather conditions into VTCCL on the nuScenes validation set, considering the following scenarios:
(1) only sunny condition;
(2) sunny condition and night; 
(3) sunny condition and rainy day;
(4) all weather.
Our results demonstrate that combining all weather conditions in VTCCL allows MMD-LoRA to achieve the best performance, consistently outperforming the other three alternatives.
When using only sunny conditions in VTCCL,  MMD-LoRA improves depth estimation for sunny and rainy conditions but degrades performance at night. 
This is because the semantic information of "sunny condition" ("an image taken during the day") and "rainy day" ("an image taken on a rainy day") share similarities (\ie "day"), whereas night-specific semantics ("an image taken at night") are not incorporated into Eq.~\ref{gongshi5}.
Similarly, when using sunny and rainy conditions in VTCCL, the results align with the earlier conclusion, showing performance improvements for those conditions but limitations for nighttime scenarios. 
Moreover, by introducing both sunny and night conditions into Eq.~\ref{gongshi5}, MMD-LoRA achieves results comparable to those obtained by combining all weather conditions, maintaining strong performance across most metrics.
These findings validate that the proposed VTCCL is well-suited for distinguishing between different weather types, enabling effective multi-modal alignment and improving depth estimation under diverse conditions.
